# Supplementary material for: Do Differentiable Simulators Give Better Policy Gradients?
Source: arXiv:2202.00817 source file (2022-08-22)
Supplement: Supplementary file 1 [file details_for_simulation.tex]

\section{Simulation Details}
\subsection{Stiffness and Implicit Time-Stepping}
Throughout our work, we define stiffness
