# Supplementary material for: Do Differentiable Simulators Give Better Policy Gradients?
Source: arXiv:2202.00817 source file (2022-08-22)
Supplement: Supplementary file 2 [file simdetails.tex]

%!TEX root = ../icml_main.tex

\section{Details of Simulation}
