# Supplementary material for: Do Differentiable Simulators Give Better Policy Gradients?
Source: arXiv:2202.00817 source file (2022-08-22)
Supplement: Supplementary file 3 [file technicalities.tex]

%!TEX root = ../icml_main.tex

\section{Technicalities}
To define the \foeg of possibly non-smooth functions, we require a rigorous definition of expectation. We refer the reader to \mscomment{...} to common definitions in real analysis (e.g. measurable function,  measure zero sets). 

Consider a function $g: \R^d \to \R^p \cup \{\bot\}$, where $g$ may take a non-vector valued function $\bot$, in addition to vector-values in $\R^p$. We say that $g$ is \emph{defined almost everywhere} if the set $\{z \in \R^d: g(x) = \bot\}$ has Lebesgue measure zero.
